# Supplementary material for: Numerical Simulation of Microflows using Hermite Spectral Methods
Source: arXiv:1807.06236 source file (2019-02-24)
Supplement: Supplementary file 1 [file article_appendix.tex]

% vim: tw=70:spell
\appendix
\section{Proof of Theorem \ref{thm:coeA}}
\label{sec:thm_proof}

In order to prove Theorem \ref{thm:coeA}, we first introduce the lemma
below:
\begin{lemma}
\label{thm:Hermit_cv}
Let $\bv = \bh + \bg/2$ and $\bw = \bh - \bg/2$. It holds that
\begin{displaymath}
\begin{split}
& H^{k_1 k_2 k_3}(\bv) H^{l_1 l_2 l_3}(\bw) = \\
& \quad \sum_{k_1'+l_1' = k_1+l_1}
  \sum_{k_2'+l_2' = k_2+l_2} \sum_{k_3'+l_3' = k_3+l_3}
  a_{k_1'l_1'}^{k_1 l_1} a_{k_2'l_2'}^{k_2 l_2} a_{k_3'l_3'}^{k_3 l_3}
  H^{k_1' k_2' k_3'}(\sqrt{2}\bh)
  H^{l_1' l_2' l_3'} \left( \frac{\bg}{\sqrt{2}} \right),
\end{split}
\end{displaymath}
where the coefficients $a_{k_s'l_s'}^{k_s l_s}$, $s = 1,2,3$ are
defined in \eqref{eq:coea}.
\end{lemma}

{
  \begin{proof}
    First, it is easy to verify that
    $ \exp\left(-\frac{|\bv|^2 + |\bw|^2}{2}\right) =
    \exp\left(-\left(|\bh|^2 + \frac{|\bg|^2}{4}\right)\right)$
    and $\dd\bv\dd \bw = \dd \bg \dd \bh$. Based on the orthogonality
    of the Hermite polynomials \eqref{eq:Her_orth}, we just need to
    prove
    \begin{equation} \label{eq:zeta_a}
    \czeta = \left\{ \begin{array}{ll}
      k_1'! k_2'! k_3'! l_1'! l_2'! l_3'!
      a_{k_1'l_1'}^{k_1 l_1} a_{k_2'l_2'}^{k_2 l_2}a_{k_3'l_3'}^{k_3 l_3},
        & \text{if } k_s + l_s = k_s' + l_s', \quad \forall s=1,2,3,
	\\
      0, & \text{otherwise},
    \end{array} \right.
    \end{equation}
    where the left hand side is defined as
    \begin{equation}
      \label{eq:coeH}
      \begin{aligned}
        \czeta := & \int_{\bbR^3}\int_{\bbR^3}
        H^{k_1 k_2 k_3}(\bv) H^{l_1 l_2 l_3}(\bw)
        H^{k_1' k_2' k_3'}(\sqrt{2}\bh) H^{l_1' l_2' l_3'} \left(
          \frac{\bg}{\sqrt{2}} \right) \exp\left(-\frac{|\bv|^2 +
            |\bw|^2}{2}\right) \dd \bv \dd \bw.
      \end{aligned}
    \end{equation}
    By the general Leibniz rule, we have the following relation for
    the derivatives of with respect to $\bv, \bw$ and $\bg, \bh$:
    \begin{equation}
      \label{eq:bin_diff}
      \frac{\partial^{k_s + l_s}}{\partial v_s^{k_s}\partial w_s^{l_s}} = 
      \sum_{i_s =0}^{k_s}\sum_{j_s=0}^{l_s}\binom{k_s}{i_s}\binom{l_s}{j_s}
      \frac{(-1)^{l_s - j_s}}{2^{i_s+j_s}}
      \frac{\partial^{k_s}}{\partial
        h_s^{i_s+j_s}}\frac{\partial^{l_s}}{\partial g_s^{i'_s+j'_s}}, \qquad
      i'_s = k_s - i_s, \quad j'_s = l_s - j_s, \quad s   = 1, 2, 3.
    \end{equation}
    Then, following the definition of Hermite polynomials
    \eqref{eq:basis} and \eqref{eq:bin_diff}, and using integration
    by parts, we arrive at
    \begin{equation}
      \label{eq:coeH_detail}
      \begin{aligned}
        & \czeta = \int_{\bbR^3}\int_{\bbR^3}
        \exp\left(-\left(|\bh|^2+\frac{|\bg|^2}{4}\right)\right) \times \\
        & \qquad \prod_{s=1}^3\left(\sum_{i_s
            =0}^{k_s}\sum_{j_s=0}^{l_s}\binom{k_s}{i_s}\binom{l_s}{j_s}
          \frac{(-1)^{l_s - j_s}}{2^{i_s+j_s}}\frac{ \partial^{k_s + l_s}
          }{\partial h_s^{i_s+j_s}\partial g_s^{i'_s+j'_s}} \right)H^{k_1'
          k_2' k_3'}(\sqrt{2}\bh)H^{l_1' l_2' l_3'}
        \left(\frac{\bg}{\sqrt{2}} \right) \dd \bh \dd \bg.
      \end{aligned}
    \end{equation}
    From the orthogonality of Hermite polynomials and the
    differentiation relation
    \begin{equation} \label{eq:Hermite_diff}
    \frac{\partial}{\partial v_s} H^{k_1 k_2 k_3}(\bv) = \left\{
      \begin{array}{ll}
      0, & \text{if } k_s = 0, \\
      k_s H^{k_1-\delta_{1s}, k_2-\delta_{2s}, k_3-\delta_{3s}}(\bv),
        & \text{if } k_s > 0,
      \end{array}
    \right.
    \end{equation}
    it holds that \eqref{eq:coeH_detail} is nonzero only when $i_s +
    j_s = k'_s$, $i'_s + j'_s = l'_s$, $s = 1,2,3$, which means
    \begin{equation}
      \label{eq:index_H}
      k_s + l_s = k'_s + l'_s, \qquad \forall s = 1,2,3.
    \end{equation}
    When \eqref{eq:index_H} holds, we can apply
    \eqref{eq:Hermite_diff} to \eqref{eq:coeH_detail} and get
      \begin{equation}
        \label{eq:coeH_detail1}
        \begin{aligned}
          \frac{\czeta}{
            k'_1!k'_2!k'_3!l'_1!l'_2!l'_3!}  & =
          \prod_{s=1}^3\left(\sum_{i_s =0}^{k_s}\sum\limits_{j_s=0,
              i_s + j_s = k'_s}^{l_s}\binom{k_s}{i_s}\binom{l_s}{j_s}
            \frac{(-1)^{l'_s - k_s + i_s}}{2^{k'_s}} 2^{\frac{k'_s -
                l'_s}{2}}\right) = a_{k_1'l_1'}^{k_1 l_1}
          a_{k_2'l_2'}^{k_2 l_2} a_{k_3'l_3'}^{k_3 l_3}.
        \end{aligned}
      \end{equation}
    Thus \eqref{eq:zeta_a} is shown, which completes the proof of the
    lemma.
  \end{proof}
}

\begin{corollary}
  \label{thm:Hermit_split}
  Let $\bv = \bh + \bg/2$. We have
  \begin{displaymath}
    H^{k_1 k_2 k_3}(\bv) = \sum_{l_1 + m_1 = k_1}
    \sum_{l_2 + m_2 = k_2} \sum_{l_3 + m_3 = k_3}
    \frac{2^{-k/2} k_1! k_2! k_3!}{l_1! l_2! l_3! m_1! m_2! m_3!}
    H^{l_1 l_2 l_3}(\sqrt{2} \bh)
    H^{m_1 m_2 m_3} \left( \frac{\bg}{\sqrt{2}} \right).
  \end{displaymath}
\end{corollary}
{ 
  \begin{proof}
  This corollary is just a special case of Lemma \ref{thm:Hermit_cv}
  when $l_1 = l_2 = l_3 = 0$.
  \end{proof}
}

{
  \begin{proof}
    Let $\bw = \bv', \bw_1 = \bv'_1, \bs = \bw - \bw_1$ and define the
    unit vector $\tilde{\bn}$ as $\tilde{\bn} = -(\bg\sin\chi /|\bg| +
    \bn\cos\chi)$. It holds that
    \begin{equation}
      \begin{gathered}
        \label{eq:conser_v}
        |\bv|^2 + |\bv_1|^2 = |\bw|^2 +
        |\bw_1|^2, \qquad \dd \bv\dd \bv_1 = \dd \bw \dd \bw_1, \qquad
        |\bs|= |\bg|, \qquad \bs \cdot \bn_{\bw} = 0, \\
        \bw' = \cos^2(\chi/2) \bw + \sin^2(\chi/2) \bw_1 -
        |\bs| \cos(\chi/2)\sin(\chi/2) \bn_{\bw} = \bv, \\
      \end{gathered}
    \end{equation}
    Following \eqref{eq:conser_v}, and by change of variables, we arrive
    at
      \begin{equation}
        \label{eq:partA}
        \begin{aligned}
          &\int_{\mathbb{R}^3} \int_{\mathbb{R}^3} \int_{\bn \perp \bg}
          \int_0^{\pi} B(|\bg|,\chi)
          H^{\newindex{i}}(\bv') H^{\newindex{j}}(\bv'_1) H^{\indexk}(\bv) \exp
          \left( -\frac{|\bv|^2 + |\bv_1|^2}{2} \right) \,\mathrm{d}\chi
          \,\mathrm{d}\bn \,\mathrm{d}\bv_1 \,\mathrm{d}\bv  \\
          ={} & \int_{\mathbb{R}^3} \int_{\mathbb{R}^3} \int_{\tilde{\bn} \perp
            \bs} \int_0^{\pi} B(|\bs|,\chi)
          H^{\newindex{i}}(\bw) H^{\newindex{j}}(\bw_1) H^{\indexk}(\bw') \exp
          \left( -\frac{|\bw|^2 + |\bw_1|^2}{2} \right) \,\mathrm{d}\chi
          \,\mathrm{d}\tilde{\bn} \,\mathrm{d}\bw_1 \,\mathrm{d}\bw \\
          ={} &\int_{\mathbb{R}^3} \int_{\mathbb{R}^3} \int_{\bn \perp \bg}
          \int_0^{\pi} B(|\bg|,\chi)
          H^{\newindex{i}}(\bv) H^{\newindex{j}}(\bv_1) H^{\indexk}(\bv') \exp
          \left( -\frac{|\bv|^2 + |\bv_1|^2}{2} \right) \,\mathrm{d}\chi
          \,\mathrm{d}\bn \,\mathrm{d}\bv_1 \,\mathrm{d}\bv.
        \end{aligned}
      \end{equation}
    Thus, we can substitute the above equality into
    \eqref{eq:coeA_detail} to get
    \begin{equation}
      \label{eq:coeA_detail1}
      \begin{aligned}
        A_{k_1k_2k_3}^{\newindex{i}, \newindex{j}} =
        &\frac{1}{(2\pi)^3\factorialk} \int_{\mathbb{R}^3}
        \int_{\mathbb{R}^3} \int_{\bn \perp \bg} \int_0^{\pi} B(|\bg|,\chi)
        [H^{k_1 k_2 k_3}(\bv') - H^{k_1 k_2k_3}(\bv)] \\
        & \qquad H^{\newindex{i}}(\bv) H^{\newindex{j}}(\bv_1) \exp
        \left(
          -\frac{|\bv|^2 + |\bv_1|^2}{2} \right) \,\mathrm{d}\chi
        \,\mathrm{d}\bn \,\mathrm{d}\bv_1 \,\mathrm{d}\bv.
      \end{aligned}
    \end{equation}
    Further simplification of \eqref{eq:coeA_detail1} follows the
    method in \cite{Grad}, where the velocity of the mass center is
    defined as $\bh = (\bv+\bv_1)/2 = (\bv' + \bv'_1)/2$. Hence,
    \begin{gather}
      \label{eq:var_change}
      \bv = \bh + \frac{1}{2} \bg, \quad
      \bv_1 = \bh - \frac{1}{2} \bg, \quad
      \bv' = \bh + \frac{1}{2} \bg', \quad
      \bv_1' = \bh - \frac{1}{2} \bg', \\
      \label{eq:gh}
      |\bv|^2 + |\bv_1|^2 = \frac{1}{2} |\bg|^2 + 2|\bh|^2, \qquad
      \mathrm{d}\bv \, \mathrm{d}\bv_1 = \mathrm{d}\bg \, \mathrm{d}\bh.
    \end{gather}
    Combining Lemma \ref{thm:Hermit_cv}, Corollary \ref{thm:Hermit_split}
    and \eqref{eq:gh}, we can rewrite \eqref{eq:coeA_detail1} as an
    integral with respect to $\bg$ and $\bh$:
    \begin{equation}
      \label{eq:coeA_detail2}
      \begin{aligned}
        A_{k_1k_2k_3}^{\newindex{i}, \newindex{j}} = &
        \sum\limits_{i'_1+j'_1=i_1+j_1}\sum\limits_{i'_2+j'_2=i_2+j_2}\sum\limits_{i'_3+j'_3=i_3+j_3}
        \sum\limits_{l'_1+k'_1=k_1}\sum\limits_{l'_2+k'_2=k_2}\sum\limits_{l'_3+k'_3=k_3}
        \\ & \qquad \frac{
          2^{-k/2}}{(2\pi)^3}\frac{1}{k_1'k_2'k_3'l'_1!l'_2!l'_3!}
        a_{i'_1j'_1}^{i_1j_1}a_{i'_2j'_2}^{i_2j_2}
        a_{i'_3j'_3}^{i_3j_3}\gamma_{j'_1j'_2j'_3}^{l'_1l'_2l'_3}\eta_{i'_1i'_2i'_3}^{k'_1k'_2k'_3},
      \end{aligned}
    \end{equation}
    where the coefficients $\gamma_{j'_1j'_2j'_3}^{l'_1l'_2l'_3}$
    defined in \eqref{eq:coe_gamma} are integrals with respect to
    $\bg$, and $\eta_{i'_1 i'_2 i'_3}^{k'_1 k'_2 k'_3}$ are integrals
    with respect to $\bh$ defined by
    \begin{equation}
      \label{eq:eta}
      \eta_{i'_1 i'_2 i'_3}^{k'_1 k'_2 k'_3} = \int_{\mathbb{R}^3}
      H^{i'_1 i'_2 i'_3} (\sqrt{2} \bh) H^{k'_1 k'_2 k'_3} (\sqrt{2} \bh)
      \exp (-|\bh|^2) \,\mathrm{d}\bh =
      \pi^{3/2} k'_1! k'_2! k'_3! \delta_{i'_1 k'_1} \delta_{i'_2 k'_2}
      \delta_{i'_3 k'_3}.
    \end{equation}
    Thus the theorem is proven by substituting \eqref{eq:eta} into
    \eqref{eq:coeA_detail2}.
  \end{proof}
}

\section{Proof of Theorem \ref{thm:gamma}}
We will first prove Theorem \ref{thm:gamma} based on
several lemmas, and then prove these lemmas. 
\subsection {Proof of Theorem \ref{thm:gamma}} 
In order to prove Theorem \ref{thm:gamma}, we will introduce the
definition of Ikenberry polynomials \cite{Ikenberry1955} and several
lemmas.
\begin{definition}[Ikenberry polynomials] \label{def:hhp}
  Let $\bv = (v_1, v_2, v_3)^T \in \mathbb{R}^3$. For
  $\forall n \in \bbN$, and $i_1, \cdots, i_n \in \{1,2,3\}$, define
  $Y_{i_1 \cdots i_n}(\bv)$ as the Ikenberry polynomials 
\begin{gather*}
  Y(\bv) = 1, \qquad Y_{i_1}(\bv) =  v_{i_1}, \\
  Y_{i_1 \cdots i_n}(\bv) = v_{i_1}\cdots v_{i_n} +
  |\bv|^2S_{n-2}^{i_1\cdots i_n}(\bv) + |\bv|^4S_{n-4}^{i_1\cdots i_n}
  + \cdots + |\bv|^{2\lfloor n/2 \rfloor}S_{n-2\lfloor n/2
    \rfloor}^{i_1\cdots i_n}(\bv),
\end{gather*}
where $S_{j}^{i_1\cdots i_n}$ is a homogeneous harmonic polynomial of
degree $j$ defined in \cite{Ikenberry1955}, which can be determined by
\begin{equation*}
  \Delta_{\bv}Y_{i_1\cdots i_n} = \Delta_{\bv}^2Y_{i_1\cdots i_n} =
  \Delta_{\bv}^{\lfloor n/2 \rfloor}Y_{i_1\cdots i_n} = 0. 
\end{equation*}
%Y_{i_1 \cdots i_n}(\bv) = v_{\langle i_1} \cdots v_{i_n \rangle},
%\end{displaymath}
%which is the trace-free part of the $n$-tensor
%$v_{i_1} \cdots v_{i_n}$
For $k_1, k_2, k_3 \in \mathbb{N}$, define $Y^{k_1 k_2 k_3}(\bv)$ as
the polynomial $Y_{i_1 \cdots i_n}(\bv)$ with
\begin{gather*}
n = k_1 + k_2 + k_3, \quad i_1 = \cdots = i_{k_1} = 1, \\
i_{k_1+1} = \cdots = i_{k_1+k_2} = 2, \quad
i_{k_1+k_2+1} = \cdots = i_n = 3.
\end{gather*}
\end{definition}
\begin{lemma}
\label{thm:S_harmonic}
The integral
\begin{displaymath}
\int_{\mathbb{S}^2} Y^{k_1 k_2 k_3}(\bn) Y^{l_1 l_2 l_3}(\bn) \,\mathrm{d}\bn
\end{displaymath}
is the coefficient of $v_1^{k_1} v_2^{k_2} v_3^{k_3} w_1^{l_1}
w_2^{l_2} w_3^{l_3}$ in the polynomial
\begin{displaymath}
\frac{4\pi}{2k+1} \frac{k_1! k_2! k_3! l_1! l_2! l_3!}{[(2k-1)!!]^2}
(|\bv| |\bw|)^k P_k \left(
  \frac{\bv}{|\bv|} \cdot \frac{\bw}{|\bw|}
\right), \qquad k = k_1 + k_2 + k_3.
\end{displaymath}
\end{lemma}
\begin{lemma}
  \label{thm:Hermite_Harmonic}
  The Hermite polynomial $H^{k_1 k_2 k_3}(\bv)$ can be represented as
  \begin{displaymath}
    \begin{split}
      H^{k_1 k_2 k_3}(\bv) &=
      \sum_{m_1=0}^{\lfloor k_1/2 \rfloor}
      \sum_{m_2=0}^{\lfloor k_2/2 \rfloor}
      \sum_{m_3=0}^{\lfloor k_3/2 \rfloor}
      \frac{(-1)^m m! (2k-4m+1)!!} {(2(k-m)+1)!!}
      \left( \prod_{i=1}^3 \frac{k_i!}{m_i! (k_i-2m_i)!} \right) \\
      &\qquad L_m^{(k-2m+1/2)} \left( \frac{|\bv|^2}{2} \right) 
      Y^{k_1-2m_1,k_2-2m_2,k_3-2m_3}(\bv),
    \end{split}
  \end{displaymath}
  where $k = k_1 + k_2 + k_3$ and $m = m_1 + m_2 + m_3$.
\end{lemma}

\begin{lemma}
  \label{thm:int_n}
  Given a vector $\bg$ and $\chi \in [0, \pi]$, let
  $\bg'(\bn) = \bg \cos \chi - |\bg| \bn \sin \chi$, where $\bn$ is a unit
  vector. It holds that
  \begin{displaymath}
    \int_{\bn \perp \bg} Y^{k_1 k_2 k_3}(\bg' / |\bg|) \,\mathrm{d}\bn
    = 2\pi Y^{k_1 k_2 k_3}(\bg / |\bg|) P_k(\cos \chi),
  \end{displaymath}
  where $k = k_1 + k_2 + k_3$ and $P_k$ is Legendre polynomial.
\end{lemma}

In above lemmas, Lemma \ref{thm:S_harmonic} and Lemma
\ref{thm:Hermite_Harmonic} will be proved in Appendix
\ref{sec:S_harmonic} and \ref{sec:Hermite_Harmonic}
respectively. Lemma \ref{thm:int_n} is proved in \cite{Ikenberry1956}.
By Lemma \ref{thm:Hermite_Harmonic} and Lemma
\ref{thm:int_n}, we can derive the corollary below
\begin{corollary}
  \label{thm:int_H}
  Given a vector $\bg$ and $\chi \in [0, \pi]$, define $\bg'(\bn)$ the
  same as in Theorem \ref{thm:int_n}. We have
  \begin{displaymath}
    \begin{split}
      & \int_{\bn \perp \bg} H^{k_1 k_2 k_3}(\bg') \,\mathrm{d}\bn =
      2\pi \sum_{m_1=0}^{\lfloor k_1/2 \rfloor}
      \sum_{m_2=0}^{\lfloor k_2/2 \rfloor}
      \sum_{m_3=0}^{\lfloor k_3/2 \rfloor}
      \frac{(-1)^m m! (2k-4m+1)!!} {(2(k-m)+1)!!} \times \\
      & \quad \left( \prod_{i=1}^3 \frac{k_i!}{m_i! (k_i-2m_i)!} \right)
      L_n^{(k-2m+1/2)} \left( \frac{|\bg|^2}{2} \right) 
      Y^{k_1-2m_1,k_2-2m_2,k_3-2m_3}(\bg) P_{k-2m}(\cos \chi),
    \end{split}
  \end{displaymath}
  where $k = k_1 + k_2 + k_3$, $m = m_1 + m_2 + m_3$.
\end{corollary}

{
\begin{proof}

  By Lemma \ref{thm:Hermite_Harmonic}, the corollary \ref{thm:int_H}
  and the homogeneity of the Ikenberry polynomials 
% \begin{equation}
%   \label{eq:harmonic}
%   Y^{\indexk}(\bg) = |\bg|^{k}Y^{\indexk}(\bg/ |\bg|), \qquad k = k_1 + k_2 + k_3, 
% \end{equation}
  $ \gamma_{\indexk}^{\indexl}$ defined in \eqref{eq:gamma} can
    be simplified as
% \begin{equation}
%   \label{eq:gmma_detail1}
%   \begin{aligned}
%     \gamma_{\indexk}^{\indexl} & = 2\pi \sum_{m_1=0}^{\lfloor k_1/2
%       \rfloor} \sum_{m_2=0}^{\lfloor k_2/2 \rfloor}
%     \sum_{m_3=0}^{\lfloor k_3/2 \rfloor}\sum_{n_1=0}^{\lfloor l_1/2
%       \rfloor} \sum_{n_2=0}^{\lfloor l_2/2 \rfloor}
%     \sum_{n_3=0}^{\lfloor l_3/2 \rfloor}
%     \frac{(2(k-m)+1)!!C_{\indexm}^{\indexk}}{4\pi\prod_{i=1}^3
%       (k_i-2m_i)!}\frac{(2(l-n)+1)!!C_{\indexn}^{\indexl}}{4\pi\prod_{i=1}^3
%       (l_i-2n_i)!}  \\
%     & \qquad \int_{\mathbb{R}^3} \int_0^{\pi}
%     Y^{k_1-2m_1,k_2-2m_2,k_3-2m_3}\left(\frac{\bg}{\sqrt{2}}\right)
%     Y^{l_1-2n_1,l_2-2n_2,l_3-2n_3}\left(\frac{\bg}{\sqrt{2}}\right)\\
%     & \qquad \qquad L_n^{(k-2m+1/2)}\left( \frac{g^2}{4} \right)L_n^{(l-2n+1/2)}
%     \left( \frac{g^2}{4} \right) (P_{k-2m}(\cos \chi)- 1) \exp\left(
%       -\frac{g^2}{4} \right) \,\mathrm{d}\chi \,\mathrm{d}\bg,
%   \end{aligned}
% \end{equation}
{\small 
  \begin{equation}
    \label{eq:gamma_detail2}
    \begin{aligned}
      \gamma_{\indexk}^{\indexl} & = 2\pi \sum_{m_1=0}^{\lfloor k_1/2
        \rfloor} \sum_{m_2=0}^{\lfloor k_2/2 \rfloor}
      \sum_{m_3=0}^{\lfloor k_3/2 \rfloor}\sum_{n_1=0}^{\lfloor l_1/2
        \rfloor} \sum_{n_2=0}^{\lfloor l_2/2 \rfloor}
      \sum_{n_3=0}^{\lfloor l_3/2 \rfloor}
      \frac{(2(k-m)+1)!!C_{\indexm}^{\indexk}}{4\pi\prod_{i=1}^3
        (k_i-2m_i)!}\frac{(2(l-n)+1)!!C_{\indexn}^{\indexl}}{4\pi\prod_{i=1}^3
        (l_i-2n_i)!} \times \\
      & \qquad 2\int_{0}^{+\infty} \int_0^{\pi}\int_{\bbS^2}
      Y^{k_1-2m_1,k_2-2m_2,k_3-2m_3}(\bn)
      Y^{l_1-2n_1,l_2-2n_2,l_3-2n_3}(\bn)\left( \frac{g}{\sqrt{2}} \right)^{k+l+2-2(m+n)} \times \\
      & \qquad \qquad L_m^{(k-2m+1/2)}\left( \frac{g^2}{4} \right)L_n^{(l-2n+1/2)}
      \left( \frac{g^2}{4} \right) B(g, \chi)\Big[P_{k-2m}(\cos \chi)- 1\Big] \exp\left(
        -\frac{g^2}{4} \right) \dd \bn \,\mathrm{d}\chi\,\mathrm{d}g,
    \end{aligned}
  \end{equation}
}
where $C_{\indexm}^{\indexl}$ is defined in \eqref{eq:coeC}.

% From Lemma \ref{thm:S_harmonic}, it holds that only when $l = m$,
% $S_{\indexk}^{\indexl}$ defined in Theorem \ref{thm:gamma} is nonzero
% which means $k - 2m = l -2n$ in \eqref{eq:gamma_detail2}. 
Substituting Lemma \ref{thm:S_harmonic} into \eqref{eq:gamma_detail2},
we complete this proof.
\end{proof}
}

\subsection{Proof of Lemma \ref{thm:S_harmonic}}
\label{sec:S_harmonic}
In order to prove Lemma \ref{thm:S_harmonic}, we first introduce the
following definitions and lemmas.
\begin{definition}[Associated Legendre functions]
  For $m = -l,\cdots,l$, the associated Legendre functions are
  defined as
  \begin{displaymath}
    P_{l}^m(x) = \frac{(-1)^m}{2^{l} l!} (1-x^2)^{m/2}
    \frac{\mathrm{d}^{l+m}}{\mathrm{d}x^{l+m}} (x^2-1)^{l}.
  \end{displaymath}
\end{definition}
\begin{definition}[Spherical harmonics]
  For $l \in \mathbb{N}$ and $m = -l, \cdots, l$, the spherical
  harmonic $Y_{l}^m(\theta, \varphi)$ is defined as
  \begin{displaymath}
    Y_{l}^m(\bn) = Y_{l}^m(\theta, \varphi) =
    \sqrt{\frac{2l+1}{4\pi} \frac{(l - m)!}{(l + m)!}}
    P_{l}^m(\cos \theta) \exp(\mathrm{i} m \varphi),
    \qquad \bn \in \mathbb{S}^2,
  \end{displaymath}
  where $(\theta,\varphi)$ is the spherical coordinates of $\bn$.
\end{definition}

\begin{lemma}[Addition theorem]
  \label{thm:addition_theorem}
  For any $l \in \mathbb{N}$, it holds that
  \begin{displaymath}
    P_{l}(\bn_1 \cdot \bn_2) = \frac{4\pi}{2l+1}
    \sum_{m=-l}^{l} Y_{l}^m(\bn_1)
    \overline{Y_{l}^m(\bn_2)},
  \end{displaymath}
  where $P_{l}$ is  Legendre polynomial.
\end{lemma}
\begin{lemma} 
  \label{thm:P=Y} 
  For any $l \in \mathbb{N}$, it holds that
  \begin{displaymath}
    (|\bv| |\bw|)^{l} P_{l} \left(
      \frac{\bv}{|\bv|} \cdot \frac{\bw}{|\bw|}
    \right) = \frac{(2l)!}{2^{l} l! l!}
    \sum_{i_1=1}^3 \cdots \sum_{i_{l}=1}^3
    w_{i_1}\cdots w_{i_{l}}
    Y_{i_1\cdots i_{l}}(\bv).
  \end{displaymath}
\end{lemma}

In the above lemmas, Lemma \ref{thm:addition_theorem} and Lemma
\ref{thm:P=Y} are well-known and their proofs can be found in
\cite{1999AmJPh} and \cite{Ikenberry1961} respectively. Based on these
two lemmas, the following corollary holds.
\begin{corollary}
  \label{thm:coe_Y}
  The harmonic polynomial $Y^{k_1 k_2 k_3}(\bv)$ is the coefficient of
  the monomial $w_1^{k_1} w_2^{k_2} w_3^{k_3}$ in the following
  polynomial of $\bw$:
  \begin{displaymath}
    \frac{k_1! k_2! k_3!}{(2k-1)!!} (|\bv| |\bw|)^k P_k \left(
      \frac{\bv}{|\bv|} \cdot \frac{\bw}{|\bw|}
    \right), \qquad k = k_1 + k_2 + k_3.
  \end{displaymath}
\end{corollary}
{
  \begin{proof}
    Since 
    \begin{displaymath}
      \sum_{i_1=1}^3 \cdots \sum_{i_{k}=1}^3
      w_{i_1}\cdots w_{i_{k}}
      Y_{i_1\cdots i_{k}}(\bv) =  \frac{k!}{k_1!k_2!k_3!}
      \sum_{k_1+k_2+k_3=k} w_1^{k_1}w_2^{k_2}w_3^{k_3}
      Y^{k_1k_2k_3}(\bv),
    \end{displaymath}
    and matching the term of $w_1^{k_1}w_2^{k_2}w_3^{k_3}$ in Lemma
    \ref{thm:P=Y}, we complete this proof.
  \end{proof}
}

{
  \begin{proof}
    % Let 
    % \begin{displaymath}
    %   C^{k_1k_2k_3} = \frac{k_1!k_2!k_3!}{(2k-1)!!}, \quad k = k_1+k_2+k_3.
    % \end{displaymath}
    From Corollary \ref{thm:coe_Y}, we can derive that
    $\int_{\mathbb{S}^2} Y^{k_1 k_2 k_3}(\bn) Y^{l_1 l_2 l_3}(\bn)
    \,\mathrm{d}\bn$
    is the coefficient of
    $v_1^{k_1}v_2^{k_2}v_3^{k_3}w_1^{l_1}w_2^{l_2} w_3^{l_3}$ in the polynomial
    \begin{displaymath}
      \int_{\mathbb{S}^2} 
      \left[\beta^{k_1k_2k_3} (|\bn| |\bv|)^kP_k\left(\bn \cdot
          \frac{\bv}{|\bv|}\right) \right]\left[\beta^{l_1l_2l_3} (|\bn|
        |\bw|)^{l}P_{l}\left(\bn \cdot
          \frac{\bw}{|\bw|}\right) \right]
      \dd \bn,
    \end{displaymath}
    where $k = k_1 + k_2 + k_3, l = l_1 + l_2 + l_3$ and
    $\beta^{\indexk} = \frac{\factorialk}{(2k-1)!!}$.  Following Theorem
    \ref{thm:addition_theorem}, it holds 
    % \begin{align*}
    %   &  \Bigg[(|\bn| |\bv|)^kP_k\left(\bn \cdot
    %     \frac{\bv}{|\bv|}\right) \Bigg]\Bigg[ (|\bn|
    %   |\bw|)^{l}P_{l}\left(\bn \cdot
    %     \frac{\bw}{|\bw|}\right) \Bigg]= \\
    %   & (|\bv| |\bw|)^k  \left(\frac{4\pi}{2k+1}\right)^2
    %   \left(\sum_{m=-k}^{k} Y_{k}^m(\bv)
    %     \overline{Y_{k}^m(\bn)}\right) \left(\sum_{n=-l}^{l} Y_{l}^n(\bn)
    %     \overline{Y_{l}^n(\bw)}\right) \\
    %   & =(|\bv| |\bw|)^k  \left(\frac{4\pi}{2k+1}\right)^2
    %   \sum_{m=-k}^{k} \sum_{n=-l}^{l}Y_{l}^n(\bn) \overline{Y_{k}^m(\bn)}
    %   Y_{k}^m(\bv)\overline{Y_{l}^n(\bw)} \\
    %   & =(|\bv| |\bw|)^k
    %   \left(\frac{4\pi}{2k+1}\right)^2
    %   \sum_{m=-k}^{k} \sum_{n=-k}^{k}Y_{k}^n(\bn)
    %   \overline{Y_{k}^m(\bn)}
    %   Y_{k}^m(\bv)\overline{Y_{k}^n(\bw)},
    % \end{align*}
    % Integrating over $\bn$, we can derive that 
    \begin{align*}
      &   \int_{\mathbb{S}^2} 
        \left[ (|\bn| |\bv|)^kP_k\left(\bn \cdot
        \frac{\bv}{|\bv|}\right) \right]\left[ (|\bn|
        |\bw|)^{l}P_{l}\left(\bn \cdot
        \frac{\bw}{|\bw|}\right) \right]
        \dd \bn \\
        % & =(|\bv|^k |\bw|)^l
        % \frac{(4\pi)^2}{(2k+1)(2l+1)}
        % \sum_{m=-k}^{k} \sum_{n=-l}^{l}  Y_{k}^m(\bv)
        % \overline{Y_{l}^n(\bw)}\int_{\mathbb{S}^2}
        % Y_{l}^n(\bn) \overline{Y_{k}^m(\bn)} \dd \bn  \\
      & =(|\bv|^k |\bw|)^l
        \frac{(4\pi)^2}{(2k+1)(2l+1)}
        \sum_{m=-k}^{k} \sum_{n=-l}^{l}  Y_{k}^m(\bv)
        \overline{Y_{l}^n(\bw)}\delta_{lk}\delta_{mn} \\
        % & =(|\bv| |\bw|)^k
        % \left(\frac{4\pi}{2k+1}\right)^2
        % \sum_{m=-k}^{k} Y_{k}^m(\bv)
        % \overline{Y_{k}^m(\bw)} \\
      & = \frac{4\pi\delta_{kl}}{2k+1}(|\bv| |\bw|)^k
        P_k\left(\frac{\bv}{|\bv|} \cdot
        \frac{\bw}{|\bw|}\right).
    \end{align*}
    Thus if $k = l$, this corollary is proved. If $k \neq l$, we can
    deduce that
    $\int_{\mathbb{S}^2} Y^{k_1 k_2 k_3}(\bn) Y^{l_1 l_2 l_3}(\bn)
    \,\mathrm{d}\bn = 0$.
    In this case, the coefficient of
    $v_1^{k_1}v_2^{k_2}v_3^{k_3}w_1^{l_1}w_2^{l_2} w_3^{l_3}$ in the
    polynomial
    $(|\bv| |\bw|)^k P_k\left(\frac{\bv}{|\bv|} \cdot
      \frac{\bw}{|\bw|}\right)$
    is also zero, and this completes the proof.
  \end{proof}
}

\subsection{Proof of Lemma \ref{thm:Hermite_Harmonic}}
\label{sec:Hermite_Harmonic}
We will prove Lemma \ref{thm:Hermite_Harmonic} in this section.  
{
  \begin{proof}
    Define the homogeneous spherical harmonic
    $Z_{i_1i_2\cdots i_k}^{(k,m)}$ of degree $k-2m$ as
    \begin{equation}
      \label{eq:hsh_Z}
      Z_{i_1i_2\cdots i_k}^{(k,m)}
        = \frac{1}{k!} \sum_{\sigma \in \mathcal{S}_k}
          Y_{i_{\sigma(1)} i_{\sigma(2)} \cdots i_{\sigma(r)}}
          \delta_{i_{\sigma(r+1)} i_{\sigma(r+2)}} \cdots
	  \delta_{i_{\sigma(k-1)} i_{\sigma(k)}},  
    \end{equation}
    where $r = k - 2m$ and the sum is taken over all permutations of
    the set $\{1,2,\cdots,k\}$, i.e.
    \begin{displaymath}
    \mathcal{S}_k = \{ \sigma \mid \sigma: \{1,2,\cdots,k\}
      \rightarrow \{1,2,\cdots,k\} \text{ is a bijection} \}.
    \end{displaymath}
    It has been proven in \cite[eqs. (3)(8)(9)(31)]{Ikenberry1962} that 
    \footnote{In \cite{Ikenberry1962}, the definition of the Laguerre
    polynomial differs from Definition \ref{def:Laguerre} by a
    constant, which makes the coefficient in our paper slightly
    different from the one in \cite{Ikenberry1962}.}
    \begin{equation}
      \label{eq:Hermit_split}
      H^{k_1k_2k_3}(\bv) =
      \sum_{m=0}^{\lfloor k/2 \rfloor}
      \frac{(-1)^mk!(2k - 4m +1)!!}{(k-2m)!(2k-2m+1)!!}
      L_m^{(k-2m+1/2)} \left( \frac{|\bv|^2}{2} \right) 
      Z^{(k,m)}_{i_1i_2\cdots i_k}(\bv),
    \end{equation}
    where the indices $i_1, \cdots, i_k$ satisfy:
    \begin{displaymath}
    i_1 = \cdots = i_{k_1} = 1, \qquad
    i_{k_1+1} = \cdots = i_{k_1+k_2} = 2, \qquad
    i_{k_1+k_2+1} = \cdots = i_k = 3.
    \end{displaymath}

    To prove Lemma \ref{thm:Hermite_Harmonic}, we just need to provide
    a more explicit expression for \eqref{eq:hsh_Z}. In order that the
    summand in \eqref{eq:hsh_Z} is nonzero, the two indices of every
    Kronecker symbol must be the same. When all the Kronecker symbols
    take $2m_1$ ones, $2m_2$ twos and $2m_3$ threes as their indices,
    the summand will actually be $Y^{k_1-2m_1, k_2-2m_2,
    k_3-2m_3}(\bv)$ according to Definition \ref{def:hhp}. Apparently
    $(m_1, m_2, m_3)$ must be indices from the following set:
    \begin{displaymath}
    \mathcal{M}_{k_1k_2k_3}^m = \{(m_1, m_2, m_3) \mid
      m_1 + m_2 + m_3 = m, \, 2m_1 \leqslant k_1, \,
      2m_2 \leqslant k_2, \, 2m_3 \leqslant k_3 \}.
    \end{displaymath}

    Next, we are going to count how many times $Y^{k_1-2m_1, k_2-2m_2,
    k_3-2m_3}(\bv)$ appears in the sum in \eqref{eq:hsh_Z}. This can
    be observed by noting that
    \begin{enumerate}
    \item The $m$ Kronecker symbols choosing from $m_1$ pairs of ones,
      $m_2$ pairs of twos and $m_3$ pairs of threes gives a factor
      $m! / (m_1! m_2! m_3!)$;
    \item The $k-2m$ indices of $Y$ choosing from $k_1-2m_1$ ones,
      $k_2-2m_2$ twos and $k_3-2m_3$ threes gives a factor $(k-2m)! /
      \big( (k_1-2m_1)! (k_2-2m_2)! (k_3-2m_3)! \big)$.
    \item Permutations of $k_1$ ones, $k_2$ twos and $k_3$ threes give
      respectively factors $k_1!$, $k_2!$ and $k_3!$.
    \end{enumerate}
    Summarizing all these results, we get
    \begin{equation}
      \label{eq:Z}
      \begin{split}
        & Z^{(k,m)}_{i_1i_2\cdots i_k} = \frac{1}{k!}
	  \sum_{(m_1,m_2,m_3)\in \mathcal{M}_{k_1k_2k_3}^m}
	    \frac{(k-2m)!m!\prod\limits_{i=1}^3 k_i!}%
	      {\prod\limits_{i=1}^3 \Big( (k_i-2m_i)!m_i!\Big)}
	    Y^{k_1-2m_1, k_2-2m_2, k_3-2m_3}(\bv).
      \end{split}
    \end{equation}
    By \eqref{eq:Hermit_split} and \eqref{eq:Z}, the proof is
    completed.
  \end{proof}
}
